# Supplementary material for: Parf: Adaptive Parameter Refining for Abstract Interpretation
Source: arXiv:2409.05794 source file (2024-09-09)
Supplement: Supplementary file 1 [file appendix.tex]

\section{Appendix}\label{sec:appendix}
\wzycommentinline{details of processing OSCS benchmarks.}
\begin{enumerate}
    \item remove bad projects
    \item extract \eva parameters from GNU Makefiles.
\end{enumerate}

However, due to time constraints, we can not complete experiments on the whole benchmarks, so we only selected one of the two test suites which contains 1,817 verification tasks for experiments.
